# Supplementary material for: Dynamic Partial Order Reduction for Checking Correctness against Transaction Isolation Levels
Source: arXiv:2303.12606 source file (2023-04-14)
Supplement: Supplementary file 1 [file rc-ra.tex]

\section{Axiomatic levels: Read Committed and Read Atomic.}
\label{sec:def:RA-RC}

\begin{figure}[H]
	\resizebox{\textwidth}{!}{
		\footnotesize
		\begin{tabular}{|c|c|}
			\hline &  \\
			
            \begin{subfigure}[t]{.4\textwidth}
                \centering
                \begin{tikzpicture}[->,>=stealth,shorten >=1pt,auto,node distance=1cm,
                    semithick, transform shape]
                    \node[transaction state, text=black] at (0,0)       	(t_1)           {$t_1$};
                    \node[transaction state, text=black, label={above:\textcolor{black}{$\writeVar{ }{x}$}}] at (-0.5,1.5) (t_2) {$t_2$};
                    \node[transaction state, text=black] at (2,0)       (o_1)           {$\alpha$};
                    \node[transaction state] at (1.5,1.5) (o_2) {$\beta$};
                    \path (t_1) edge[color=wrColor] node {$\wro_x$} (o_1);
                    % \path (t_2) edge[blue] node {$\CO$} (t_1);
                    \path (t_2) edge[color=wrColor] node {$\wro$} (o_2);
                    \path (o_2) edge[color=poColor] node {$\po$} (o_1);
                    \path (t_2) edge[left,double,color=coColor] node {$\co$} (t_1);
                \end{tikzpicture}
                \parbox{\textwidth}{
                    $\forall x,\ \forall t_1, t_2,\ \forall \alpha.\ t_1\neq t_2\ \land$
                    
                    \hspace{2mm}$\tup{t_1,\alpha}\in \wro_x \land \writeVar{t_2}{x}\ \land$ 
                    
                    \hspace{2mm}$\tup{t_2,\alpha}\in\wro\circ\po$
                    
                    \hspace{4mm}$\implies \tup{t_2,t_1}\in\co$
                }
                %\end{align*}
                
                \caption{$\mathsf{Read\ Committed}$}
                \label{lock_rc_def}
            \end{subfigure}   
			
			&

			\begin{subfigure}[t]{.4\textwidth}
				\centering
				\begin{tikzpicture}[->,>=stealth,shorten >=1pt,auto,node distance=1cm,
					semithick, transform shape]
					\node[transaction state, text=black] at (0,0)       (t_1)           {$t_1$};
					\node[transaction state] at (2,0)       (t_3)           {$t_3$};
					\node[transaction state, text=black,label={above:\textcolor{black}{$\writeVar{ }{\xvar}$}}] at (-.5,1.5) (t_2) {$t_2$};
					\path (t_1) edge[wrColor] node {$\wro_x$} (t_3);
					% \path (t_2) edge[blue] node {$\CO$} (t_1);
					\path (t_2) edge[bend left] node {$\so \cup \wro$} (t_3);
					\path (t_2) edge[left, double ,coColor] node {$\co$} (t_1);
				\end{tikzpicture}
				\parbox{\textwidth}{
					$\forall x,\ \forall t_1, t_2,\ \forall t_3.\ t_1\neq t_2\ \land$
					
					\hspace{2mm}$\tup{t_1,t_3}\in \wro_x \land \writeVar{t_2}{x}\ \land$ 
					
					\hspace{2mm}$\tup{t_2,t_3}\in\so \cup \wro$
					
					\hspace{4mm}$\implies \tup{t_2,t_1}\in\co$
				}
				
				\caption{$\mathsf{Read\ Atomic}$}
				\label{ra_def}
			\end{subfigure}

		\\\hline
		\end{tabular}
	}
	%  \vspace{-3mm}
	\caption{Axioms defining isolations levels. The reflexive and transitive, resp., transitive, closure of a relation $rel$ is denoted by $rel^*$, resp., $rel^+$. Also, $\circ$ denotes the composition of two relations, i.e., $rel_1 \circ rel_2 = \{\tup{a, b} | \exists c. \tup{a, c} \in rel_1 \land \tup{c, b} \in rel_2\}$.}
	\label{fig:consistency_defs_rc_ra}
	%  \vspace{-2mm}
\end{figure}

The axioms defined above in Figure~\ref{fig:consistency_defs_rc_ra} define the homonymous isolation levels \textit{Read Atomic} (also called Repeatable Read in the literature) and \textit{Read Committed}.
