# Supplementary material for: Dynamic Partial Order Reduction for Checking Correctness against Transaction Isolation Levels
Source: arXiv:2303.12606 source file (2023-04-14)
Supplement: Supplementary file 3 [file experiments.tex]

%!TEX root = main.tex
\section{Experimental data}
\label{sec:appendix:experiments}

\subsection{Application Scalability}
\label{ssec:appendix:application-scalability}

% Please add the following required packages to your document preamble:
% \usepackage{booktabs}
% \usepackage[table,xcdraw]{xcolor}
% If you use beamer only pass "xcolor=table" option, i.e. \documentclass[xcolor=table]{beamer}

\begin{table}[H]
    \resizebox{\textwidth}{!}{

    \begin{tabular}{ccccccccccccccc}
        \toprule
        & \multicolumn{4}{c}{CC}                     &  & \multicolumn{4}{c}{CC + SI}                     &  & \multicolumn{4}{c}{CC + SER}                    \\ \cline{2-5} \cline{7-10} \cline{12-15} 
        & Histories & End states & Time   & Mem.     &  & Histories & End states & Time   & Mem.     &  & Histories & End states & Time   & Mem.     \\ \hline
        courseware-1 & 216 & 216 & 00:00:22 & 370 & ~ & 81 & 216 & 00:00:25 & 370 & ~ & 72 & 216 & 00:00:23 & 370 \\ 
        courseware-2 & 46 & 46 & 00:00:06 & 316 & ~ & 34 & 46 & 00:00:06 & 308 & ~ & 34 & 46 & 00:00:06 & 314 \\ 
        courseware-3 & 12790 & 12790 & 00:12:45 & 533 & ~ & 6197 & 12790 & 00:13:59 & 533 & ~ & 960 & 12790 & 00:12:37 & 557 \\ 
        courseware-4 & 69 & 69 & 00:00:07 & 314 & ~ & 39 & 69 & 00:00:08 & 324 & ~ & 17 & 69 & 00:00:07 & 370 \\ 
        courseware-5 & 388 & 388 & 00:00:25 & 308 & ~ & 136 & 388 & 00:00:27 & 370 & ~ & 71 & 388 & 00:00:24 & 370 \\ 
        shoppingCart-1 & 444 & 444 & 00:00:19 & 308 & ~ & 108 & 444 & 00:00:22 & 308 & ~ & 81 & 444 & 00:00:19 & 308 \\ 
        shoppingCart-2 & 2934 & 2934 & 00:00:55 & 308 & ~ & 811 & 2934 & 00:01:13 & 444 & ~ & 480 & 2934 & 00:00:58 & 308 \\ 
        shoppingCart-3 & 1594 & 1594 & 00:00:55 & 308 & ~ & 1077 & 1594 & 00:01:05 & 308 & ~ & 338 & 1594 & 00:01:00 & 308 \\ 
        shoppingCart-4 & 58677 & 58677 & \red{TL}  & 444 & ~ & 12440 & 49589 & \red{TL}  & 444 & ~ & 779 & 60194 & \red{TL}  & 383 \\ 
        shoppingCart-5 & 4686 & 4686 & 00:02:56 & 444 & ~ & 1986 & 4686 & 00:03:07 & 444 & ~ & 780 & 4686 & 00:02:41 & 308 \\ 
        tpcc-1 & 165 & 165 & 00:00:43 & 794 & ~ & 47 & 165 & 00:00:47 & 808 & ~ & 47 & 165 & 00:00:45 & 796 \\ 
        tpcc-2 & 353 & 353 & 00:01:25 & 699 & ~ & 35 & 353 & 00:01:29 & 879 & ~ & 31 & 353 & 00:01:25 & 704 \\ 
        tpcc-3 & 1593 & 1593 & 00:10:12 & 966 & ~ & 232 & 1593 & 00:10:29 & 1054 & ~ & 116 & 1593 & 00:10:05 & 803 \\ 
        tpcc-4 & 105 & 105 & 00:00:15 & 450 & ~ & 22 & 105 & 00:00:16 & 485 & ~ & 1 & 105 & 00:00:15 & 396 \\ 
        tpcc-5 & 7836 & 7836 & \red{TL}  & 1732 & ~ & 695 & 6973 & \red{TL}  & 1647 & ~ & 271 & 7617 & \red{TL}  & 1640 \\ 
        twitter-1 & 36 & 36 & 00:00:05 & 256 & ~ & 29 & 36 & 00:00:06 & 308 & ~ & 18 & 36 & 00:00:05 & 256 \\ 
        twitter-2 & 876 & 876 & 00:00:48 & 459 & ~ & 263 & 876 & 00:01:03 & 1066 & ~ & 122 & 876 & 00:00:56 & 513 \\ 
        twitter-3 & 1072 & 1072 & 00:01:24 & 444 & ~ & 576 & 1072 & 00:01:33 & 569 & ~ & 216 & 1072 & 00:01:21 & 444 \\ 
        twitter-4 & 12915 & 12915 & 00:08:36 & 444 & ~ & 1680 & 12915 & 00:10:59 & 640 & ~ & 1680 & 12915 & 00:09:12 & 533 \\ 
        twitter-5 & 12915 & 12915 & 00:07:53 & 444 & ~ & 1680 & 12915 & 00:11:18 & 533 & ~ & 1680 & 12915 & 00:07:43 & 444 \\ 
        wikipedia-1 & 649 & 649 & 00:03:59 & 820 & ~ & 95 & 649 & 00:02:34 & 699 & ~ & 95 & 649 & 00:02:32 & 695 \\ 
        wikipedia-2 & 3610 & 3610 & 00:13:51 & 792 & ~ & 328 & 3610 & 00:14:13 & 696 & ~ & 292 & 3610 & 00:13:50 & 798 \\ 
        wikipedia-3 & 2339 & 2339 & 00:05:44 & 640 & ~ & 175 & 2339 & 00:06:04 & 640 & ~ & 175 & 2339 & 00:05:41 & 640 \\ 
        wikipedia-4 & 691 & 691 & 00:01:54 & 774 & ~ & 246 & 691 & 00:02:01 & 768 & ~ & 108 & 691 & 00:01:55 & 774 \\ 
        wikipedia-5 & 21317 & 21317 & \red{TL}  & 620 & ~ & 292 & 19840 & \red{TL}  & 533 & ~ & 220 & 22307 & \red{TL}  & 444 \\
        \bottomrule
    \end{tabular}
    }
\end{table}

\begin{table}[H]
    \resizebox{\textwidth}{!}{
    \begin{tabular}{ccccccccccccccccccc}
        \toprule
        & \multicolumn{4}{c}{RA + CC}                     &  & \multicolumn{4}{c}{RC + CC}                     &  & \multicolumn{4}{c}{\texttt{true} + CC}           &  & \multicolumn{3}{c}{DFS(CC)}      \\ \cline{2-5} \cline{7-10} \cline{12-15} \cline{17-19} 
        & Histories & End states & Mem.   & Time     &  & Histories & End states & Mem.   & Time     &  & Histories & End states & Mem.  & Time &  & End states & Mem.   & Time     \\ \hline
        courseware-1 & 216 & 893 & 00:00:52 & 370 & ~ & 216 & 11751 & 00:07:02 & 370 & ~ & 216 & 124399 & \red{TL} & 444 & ~ & 58072 & 00:13:52 & 308 \\ 
        courseware-2 & 46 & 106 & 00:00:06 & 308 & ~ & 46 & 588 & 00:00:11 & 308 & ~ & 46 & 1074 & 00:00:15 & 308 & ~ & 18010 & 00:02:12 & 308 \\ 
        courseware-3 & 10585 & 47570 & \red{TL} & 444 & ~ & 40 & 65075 & \red{TL} & 308 & ~ & 40 & 119388 & \red{TL} & 370 & ~ & 186758 & \red{TL} & 308 \\ 
        courseware-4 & 69 & 88 & 00:00:07 & 308 & ~ & 69 & 2392 & 00:00:29 & 308 & ~ & 69 & 3779 & 00:00:39 & 315 & ~ & 37956 & 00:07:19 & 308 \\ 
        courseware-5 & 388 & 765 & 00:00:39 & 308 & ~ & 388 & 66557 & 00:27:12 & 370 & ~ & 320 & 96681 & \red{TL} & 660 & ~ & 68074 & \red{TL} & 308 \\ 
        shoppingCart-1 & 444 & 1620 & 00:00:34 & 370 & ~ & 444 & 202066 & \red{TL} & 370 & ~ & 370 & 173904 & \red{TL} & 308 & ~ & 69396 & \red{TL} & 308 \\ 
        shoppingCart-2 & 2934 & 32976 & 00:19:58 & 450 & ~ & 366 & 224700 & \red{TL} & 370 & ~ & 366 & 508967 & \red{TL} & 370 & ~ & 93549 & \red{TL} & 308 \\ 
        shoppingCart-3 & 1594 & 6291 & 00:01:41 & 308 & ~ & 1594 & 131226 & 00:18:23 & 308 & ~ & 1594 & 223740 & \red{TL} & 308 & ~ & 99522 & \red{TL} & 533 \\ 
        shoppingCart-4 & 19945 & 53687 & \red{TL} & 533 & ~ & 151 & 256686 & \red{TL} & 308 & ~ & 11 & 267433 & \red{TL} & 308 & ~ & 270996 & \red{TL} & 370 \\ 
        shoppingCart-5 & 4686 & 16323 & 00:06:43 & 370 & ~ & 2469 & 265924 & \red{TL} & 469 & ~ & 371 & 420084 & \red{TL} & 444 & ~ & 191813 & \red{TL} & 404 \\ 
        tpcc-1 & 165 & 958 & 00:02:13 & 839 & ~ & 7 & 50588 & \red{TL} & 1045 & ~ & 3 & 84272 & \red{TL} & 545 & ~ & 18489 & \red{TL} & 1383 \\ 
        tpcc-2 & 353 & 3958 & 00:11:24 & 809 & ~ & 3 & 7029 & \red{TL} & 1153 & ~ & 1 & 23097 & \red{TL} & 670 & ~ & 25253 & \red{TL} & 1029 \\ 
        tpcc-3 & 1475 & 10969 & \red{TL} & 1029 & ~ & 20 & 22934 & \red{TL} & 688 & ~ & 2 & 119267 & \red{TL} & 459 & ~ & 18124 & \red{TL} & 1251 \\ 
        tpcc-4 & 105 & 114 & 00:00:15 & 474 & ~ & 17 & 50203 & \red{TL} & 640 & ~ & 3 & 112330 & \red{TL} & 670 & ~ & 22645 & \red{TL} & 948 \\ 
        tpcc-5 & 271 & 9178 & \red{TL} & 1629 & ~ & 3 & 4059 & \red{TL} & 662 & ~ & 3 & 48306 & \red{TL} & 768 & ~ & 36060 & \red{TL} & 1284 \\ 
        twitter-1 & 36 & 44 & 00:00:05 & 256 & ~ & 36 & 4104 & 00:01:07 & 370 & ~ & 36 & 12384 & 00:02:56 & 473 & ~ & 35056 & 00:20:25 & 533 \\ 
        twitter-2 & 876 & 2917 & 00:02:01 & 592 & ~ & 876 & 18219 & 00:09:30 & 548 & ~ & 876 & 37943 & 00:17:35 & 544 & ~ & 145070 & \red{TL} & 533 \\ 
        twitter-3 & 1072 & 2272 & 00:02:05 & 576 & ~ & 1072 & 9514 & 00:08:10 & 533 & ~ & 1072 & 20164 & 00:16:14 & 588 & ~ & 108792 & 00:24:34 & 452 \\ 
        twitter-4 & 12915 & 48363 & 00:29:09 & 476 & ~ & 10 & 114588 & \red{TL} & 370 & ~ & 1 & 147462 & \red{TL} & 533 & ~ & 50404 & \red{TL} & 533 \\ 
        twitter-5 & 12915 & 48363 & 00:27:07 & 444 & ~ & 84 & 70376 & \red{TL} & 444 & ~ & 84 & 136241 & \red{TL} & 370 & ~ & 57654 & \red{TL} & 444 \\ 
        wikipedia-1 & 649 & 2296 & 00:04:16 & 672 & ~ & 64 & 37382 & \red{TL} & 832 & ~ & 4 & 66814 & \red{TL} & 699 & ~ & 54510 & \red{TL} & 660 \\ 
        wikipedia-2 & 2049 & 8451 & \red{TL} & 979 & ~ & 17 & 19697 & \red{TL} & 795 & ~ & 2 & 85523 & \red{TL} & 930 & ~ & 43629 & \red{TL} & 650 \\ 
        wikipedia-3 & 2339 & 6170 & 00:10:06 & 640 & ~ & 100 & 28952 & \red{TL} & 522 & ~ & 50 & 23974 & \red{TL} & 581 & ~ & 43962 & \red{TL} & 682 \\ 
        wikipedia-4 & 691 & 1781 & 00:02:57 & 925 & ~ & 5 & 44937 & \red{TL} & 567 & ~ & 3 & 61334 & \red{TL} & 543 & ~ & 24873 & \red{TL} & 1188 \\ 
        wikipedia-5 & 13159 & 26384 & \red{TL} & 533 & ~ & 29 & 72930 & \red{TL} & 444 & ~ & 23 & 78413 & \red{TL} & 695 & ~ & 97881 & \red{TL} & 444 \\ 
        \bottomrule
    \end{tabular}
    }
\end{table}

\subsection{Session Scalability}
\label{ssec:appendix:session-scalability}

\begin{table}[H]
    \resizebox{\textwidth}{!}{
\begin{tabular}{cccccccccccccccccccc}
    \toprule
    &\multicolumn{3}{c}{One session}&  & \multicolumn{3}{c}{Two sessions} &  & \multicolumn{3}{c}{Three sessions} &  & \multicolumn{3}{c}{Four sessions}  &  & \multicolumn{3}{c}{Five sessions}  \\ \cline{2-4} \cline{6-8} \cline{10-12} \cline{14-16} \cline{18-20} 
    & Histories & Time   & Mem.     &  & Histories & Time   & Mem.     &  & Histories & Time   & Mem.     &  & Histories & Time   & Mem.     &  & Histories & Time   & Mem.     \\ \hline
    tpcc-1 & 1 & 00:00:02 & 256 &  & 6 & 00:00:03 & 256 &  & 1540 & 00:05:42 & 804 &  & 3081 & \red{TL} & 4096 &  & 14525 & \red{TL} & 4096 \\ 
    tpcc-2 & 1 & 00:00:03 & 256 &  & 66 & 00:00:17 & 587 &  & 9630 & \red{TL} & 2900 &  & 17637 & \red{TL} & 4076 &  & 2442 & \red{TL} & 4096 \\ 
    tpcc-3 & 1 & 00:00:03 & 256 &  & 12 & 00:00:09 & 384 &  & 4824 & 00:25:43 & 1503 &  & 3463 & \red{TL} & 4096 &  & 2940 & \red{TL} & 4096 \\ 
    tpcc-4 & 1 & 00:00:03 & 256 &  & 90 & 00:00:41 & 674 &  & 6355 & \red{TL} & 1728 &  & 1722 & \red{TL} & 4096 &  & 2634 & \red{TL} & 4096 \\ 
    tpcc-5 & 1 & 00:00:03 & 256 &  & 96 & 00:00:41 & 692 &  & 3659 & \red{TL} & 1765 &  & 1343 & \red{TL} & 4092 &  & 1481 & \red{TL} & 4096 \\ 
    wikipedia-1 & 1 & 00:00:02 & 256 &  & 199 & 00:00:19 & 370 &  & 19654 & \red{TL} & 640 &  & 16377 & \red{TL} & 533 &  & 12419 & \red{TL} & 4096 \\ 
    wikipedia-2 & 1 & 00:00:02 & 256 &  & 38 & 00:00:14 & 536 &  & 7055 & 00:22:07 & 768 &  & 21000 & \red{TL} & 3520 &  & 16985 & \red{TL} & 4096 \\ 
    wikipedia-3 & 1 & 00:00:02 & 256 &  & 67 & 00:00:14 & 444 &  & 9346 & \red{TL} & 768 &  & 9451 & \red{TL} & 4096 &  & 3264 & \red{TL} & 4096 \\ 
    wikipedia-4 & 1 & 00:00:02 & 256 &  & 7 & 00:00:07 & 374 &  & 73 & 00:00:14 & 602 &  & 3940 & 00:20:40 & 4096 &  & 1325 & \red{TL} & 4096 \\ 
    wikipedia-5 & 1 & 00:00:02 & 256 &  & 28 & 00:00:08 & 308 &  & 336 & 00:05:41 & 662 &  & 10914 & \red{TL} & 4096 &  & 563 & \red{TL} & 3936 \\ 
    \bottomrule
\end{tabular}
}
\end{table}

\subsection{Transaction Scalability}
\label{ssec:appendix:transaction-scalability}

% Please add the following required packages to your document preamble:
% \usepackage{booktabs}
% \usepackage[table,xcdraw]{xcolor}
% If you use beamer only pass "xcolor=table" option, i.e. \documentclass[xcolor=table]{beamer}

\begin{table}[H]
    \resizebox{\textwidth}{!}{
        \begin{tabular}{cccccccccccccccccccc}
        \toprule
        &\multicolumn{3}{c}{One transaction}&  & \multicolumn{3}{c}{Two transactions}   &  & \multicolumn{3}{c}{Three transactions} &  & \multicolumn{3}{c}{Four transactions}  &  & \multicolumn{3}{c}{Five transactions}  \\ \cline{2-4} \cline{6-8} \cline{10-12} \cline{14-16} \cline{18-20} 
        & Histories & Mem.   & Time     &  & Histories & Mem.   & Time     &  & Histories & Mem.   & Time     &  & Histories & Mem.   & Time     &  & Histories & Mem.   & Time     \\ \hline
        tpcc-1 & 4 & 00:00:03 & 256 & ~ & 107 & 00:00:46 & 674 & ~ & 303 & 00:01:32 & 812 & ~ & 13780 & 00:27:59 & 3904 & ~ & 13431 & \red{TL} & 4096 \\ 
        tpcc-2 & 18 & 00:00:11 & 444 & ~ & 4030 & 00:16:10 & 1063 & ~ & 5162 & \red{TL} & 2012 & ~ & 5351 & \red{TL} & 4096 & ~ & 3243 & \red{TL} & 4096 \\ 
        tpcc-3 & 3 & 00:00:04 & 256 & ~ & 219 & 00:01:38 & 881 & ~ & 6679 & \red{TL} & 1327 & ~ & 6533 & \red{TL} & 4093 & ~ & 2036 & \red{TL} & 4096 \\ 
        tpcc-4 & 20 & 00:00:13 & 444 & ~ & 5187 & 00:20:04 & 1046 & ~ & 3262 & \red{TL} & 2066 & ~ & 1548 & \red{TL} & 4096 & ~ & 2045 & \red{TL} & 4096 \\ 
        tpcc-5 & 1 & 00:00:03 & 256 & ~ & 23 & 00:00:15 & 596 & ~ & 171 & 00:01:31 & 901 & ~ & 1812 & \red{TL} & 3933 & ~ & 4091 & \red{TL} & 4096 \\ 
        wikipedia-1 & 16 & 00:00:04 & 308 & ~ & 2428 & 00:02:30 & 444 & ~ & 22289 & \red{TL} & 533 & ~ & 17113 & \red{TL} & 640 & ~ & 14648 & \red{TL} & 4096 \\ 
        wikipedia-2 & 9 & 00:00:06 & 256 & ~ & 56 & 00:00:20 & 533 & ~ & 739 & 00:02:02 & 690 & ~ & 5364 & \red{TL} & 4068 & ~ & 3568 & \red{TL} & 3977 \\ 
        wikipedia-3 & 18 & 00:00:07 & 308 & ~ & 1109 & 00:01:24 & 640 & ~ & 26110 & \red{TL} & 768 & ~ & 15339 & \red{TL} & 3621 & ~ & 15138 & \red{TL} & 3822 \\ 
        wikipedia-4 & 4 & 00:00:05 & 256 & ~ & 43 & 00:00:12 & 444 & ~ & 3919 & 00:29:57 & 1649 & ~ & 3501 & \red{TL} & 4096 & ~ & 2506 & \red{TL} & 4096 \\ 
        wikipedia-5 & 2 & 00:00:03 & 256 & ~ & 20 & 00:00:10 & 444 & ~ & 46 & 00:00:20 & 370 & ~ & 754 & 00:05:42 & 2521 & ~ & 2573 & \red{TL} & 4096 \\ 
        \bottomrule
    \end{tabular}
    }
\end{table}
